# Supplementary material for: Defining and detecting quantum speedup
Source: arXiv:1401.2910 ancillary file (2014-01-13)
Supplement: Supplementary file 1 [file supplementary.pdf]

## Supplementary material for “Defining and detecting quantum speedup”

Troels F. Rønnow,<sup>1</sup> Zhihui Wang,<sup>2</sup> Joshua Job,<sup>3</sup> Sergio Boixo,<sup>4</sup> Sergei V. Isakov,<sup>5</sup>  
David Wecker,<sup>6</sup> John M. Martinis,<sup>7</sup> Daniel A. Lidar,<sup>8</sup> and Matthias Troyer<sup>\*1</sup>

<sup>1</sup>*Theoretische Physik, ETH Zurich, 8093 Zurich, Switzerland*

<sup>2</sup>*Department of Chemistry and Center for Quantum Information Science & Technology,  
University of Southern California, Los Angeles, California 90089, USA*

<sup>3</sup>*Department of Physics and Center for Quantum Information Science & Technology,  
University of Southern California, Los Angeles, California 90089, USA*

<sup>4</sup>*Google, 150 Main St, Venice Beach, CA, 90291*

<sup>5</sup>*Google, Brandschenkestrasse 110, 8002 Zurich, Switzerland*

<sup>6</sup>*Quantum Architectures and Computation Group, Microsoft Research, Redmond, WA 98052, USA*

<sup>7</sup>*Department of Physics, University of California, Santa Barbara, CA 93106-9530, USA*

<sup>8</sup>*Departments of Electrical Engineering, Chemistry and Physics,  
and Center for Quantum Information Science & Technology,  
University of Southern California, Los Angeles, California 90089, USA*

Scaling plots for range  $r = 3$  instances, requiring 3 bits of precision in the couplings, are shown in figure 1, complementing figure 3 in the main text. Figure 2 displays the ratio of quantiles and, like figure 4 in the main text, does not exhibit a limited quantum speedup. We have obtained similar results (not shown) for ranges  $r = 2, 4, 5, 6$  and for instances including random longitudinal fields. The wall-clock results for  $r = 3$ , complementing figure 5 in the main text, are shown in figure 3.

Figure 4 shows the instance-by-instance comparisons for both the pure annealing time and the wall-clock time, with and without gauge averaging. The conclusions are very similar to those obtained based on figure 6 in the

main text using the  $r = 1, 7$  data. Figure 5 displays the results for the quantiles of ratio of time to solution. The results are intermediate between those seen in figure 7 in the main text for  $r = 1, 7$ , namely, while for  $r = 1$  there appears to be a limited quantum speedup (relative to SA) for the higher quantiles, this speedup disappears for  $r = 7$ ; for  $r = 3$  we observe a flattening of the speedup curves starting at the 75th percentile, while the lower percentiles bend down. The same suboptimality remarks discussed in this context in the main text apply. Finally, figure 6 complements figure 10 of the Methods section of the main text.

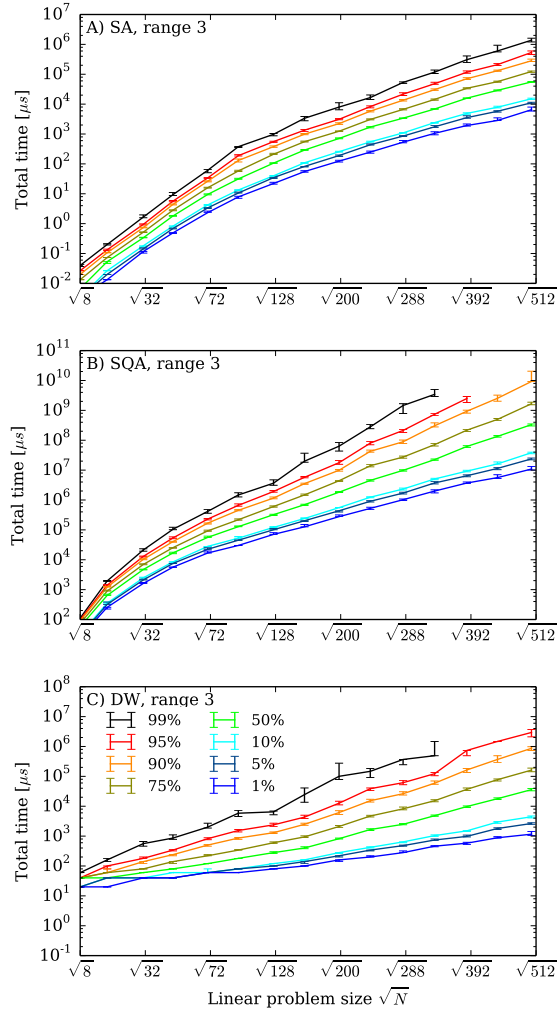

FIG. 1. **Scaling of time to solution for  $r = 3$ .** Shown is the scaling for the time to find the ground state with a probability of 99% for various quantiles of hardness for A) the simulated annealer, B) the simulated quantum annealer, and C) the DW2 device.

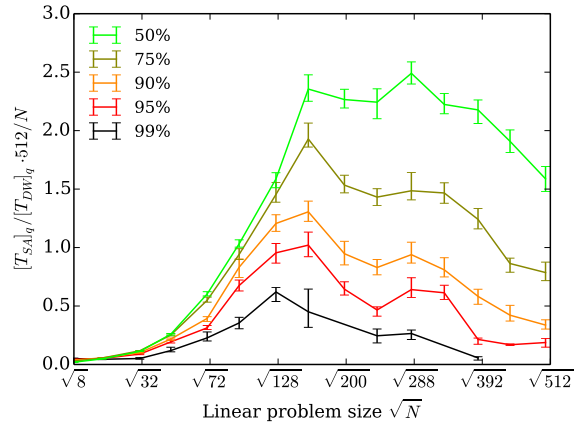

FIG. 2. **Speedup for ratio of quantiles for the DW2 device compared to SA for instances with range  $r = 3$ .** Shown are curves from the median (50th quantile) to the 99th quantile. 16 gauges were used.

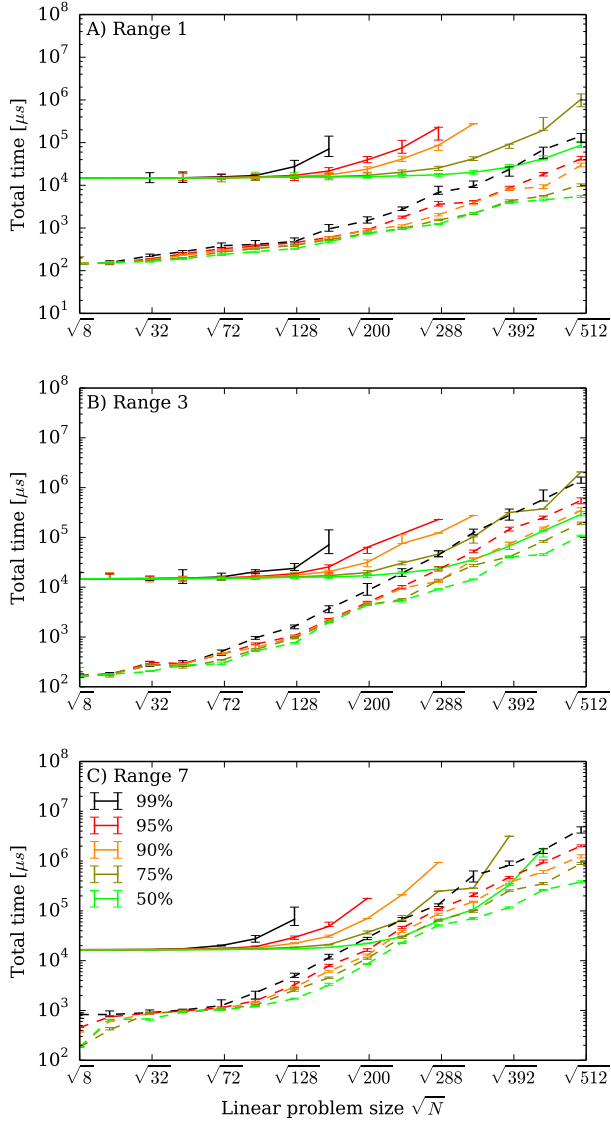

FIG. 3. **Comparing wall-clock times.** A comparison of the wall-clock time to find the solution with probability  $p = 0.99$  for SA running on a single CPU (dashed lines) compared to the DW2 [solid lines] using a single gauge choice. A) for range  $r = 1$ , B) for range  $r = 3$ , C) for range  $r = 7$ . Shown are curves from the median (50th quantile) to the 99th quantile. The large constant programming overhead of the DW2 masks the exponential increase of time to solution that is obvious in the plots of pure annealing time.

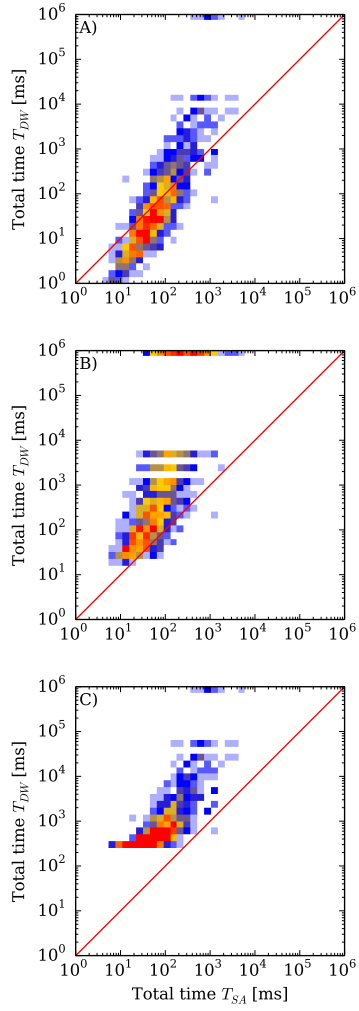

FIG. 4. **Instance-by-instance comparison.** Shown is a scatter plot of the total time for the DW2 device (DW) compared to a simulated classical annealer (SA) for  $r = 3$ . A) pure annealing time on the DW2 compared to SA using an average over 16 gauges on the DW2, B) wall-clock time using a single gauge on the DW2, C) wall-clock time using 16 gauges on the DW2. The color scale indicates the number of instances in each square. Instances below the diagonal red line are faster on the DW2, those above are faster classically. Instances for which the DW2 device did not find the solution are shown at the top. SA found a solution for every instance of this benchmark.

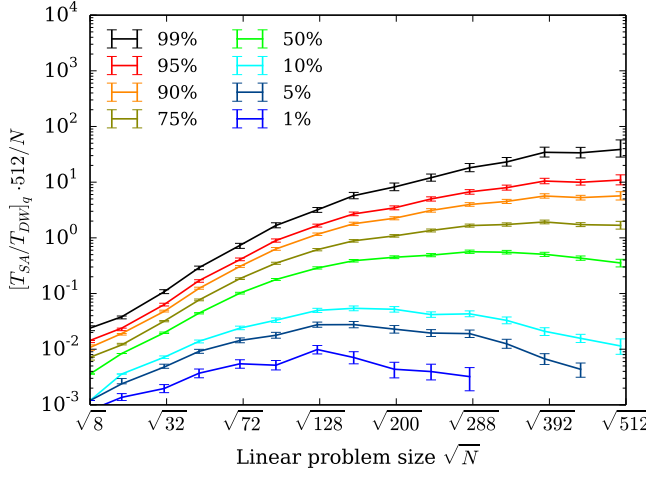

FIG. 5. **Speedup for quantiles of the ratio for  $r = 3$**  of the DW2 compared to simulated annealing. The results are intermediate between the  $r = 1$  and  $r = 7$  results as discussed in the text.

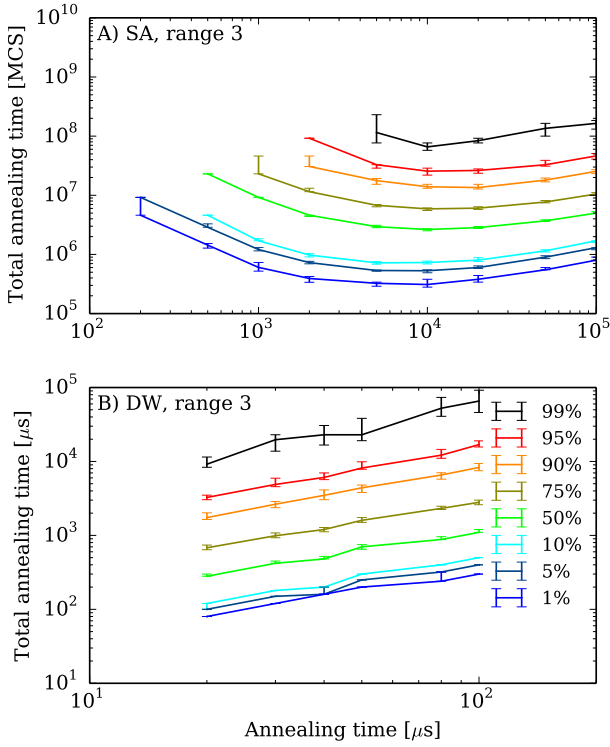

FIG. 6. **Optimal annealing times for the simulated annealer and for the D-Wave device.** Shown is the total effort  $R(t_a)t_a$  as a function of annealing time  $t_a$  for various quantiles of problems with  $r = 3$ . A) SA, where the minimum of the total effort determines the optimal annealing time  $t_a^{\text{opt}}$ . B) DW2, where we find a monotonically increasing total effort, meaning that the optimal time  $t_a^{\text{opt}}$  is always shorter than the minimal annealing time of  $20\mu\text{s}$ . This complements and agrees with the results shown in Figure 10 in the Methods section of the main text.
